# Supplementary material for: Thermodynamics education for energy transformation: a Stirling Engine experiment
Source: arXiv:2105.08142 source file (2021-05-17)
Supplement: Supplementary file 1 [file appendix.tex]

Appendix A Text
